# Supplementary material for: Partitioning Graph Databases - A Quantitative Evaluation
Source: arXiv:1301.5121 source file (2013-01-22)
Supplement: Supplementary file 1 [file 14_Appendix_neo4j_partitioned_api.tex]

\chapter{neo4j\_partitioned\_api}
\label{apx:neo4j_partitioned_api}

The neo4j\_partitioned\_api is an abstract framework on top of Neo4j v1.0 providing basic structure for a partitioned graph database. PGraphDatabaseService is an extension of GraphDatabaseService including functionality to manage partitions, adding nodes on a certain partition and retrieving information about each partition. Information about partitions are retrieved within a InstanceInfo object. The abstract classes pNodeAbs and pRelationshipAbs extend the basic Node and Relationship classes representing Edges and Vertieces in a distributed enviroment. They include the enxtended ID layer consisting of a local id (LID) a partition ID (PID) and a global ID (GID). The GIDService maps the GID of each entity in the graphdatabase to its PID/LID pair and therefore to its pysaical position.
\begin{figure}[htbp]
\begin{center}
\includegraphics[scale=1.0]{images/uml_class_diagrams/pGraphDBService.pdf} 
\caption{Simplified class diagram --- neo4j\_partitioned\_api}
\label{fig:neo4j_partitioned_api}
\end{center}
\end{figure}
